# Supplementary material for: A Co-Design Framework of Neural Networks and Quantum Circuits Towards Quantum Advantage
Source: arXiv:2006.14815 source file (2020-09-09)
Supplement: Supplementary file 1 [file appendix.pdf]

# Supplementary Information to: Can Quantum Computers Learn Like Classical Computers? A Co-Design Framework for Machine Learning and Quantum Circuits

**Weiwen Jiang[1], Jinjun Xiong[2], and Yiyu Shi[1]**

[1]University of Notre Dame, Notre Dame, IN, 46556, USA
[2]IBM Thomas J. Watson Research Center, Yorktown Heights, NY, 10598, USA

This supplementary information will first introduce the basic gates used in QF-Circ design. Based on these knowledge, we will demonstrate the equivalency between QF-Net and QF-Circ for both neural computation and batch normalization. Then, we will demonstrate the equivalency between the original circuit and optimized circuits for 2-input neural computation.

## 1 Basic Gates used in QF-Circ

In QF-Circ, there are six basic quantum gates, as shown in Figure 1(a)-(f). We also utilize a gate identity property in QF-Circ. In this section, we will show the function of each of them.

### 1.1 Y gate with parameter $\theta$

Initially, the qbit $q_0$ in Figure 1 is at $|0\rangle$ state, indicating $|q_0\rangle = 1\cdot|0\rangle + 0\cdot|1\rangle$. After applying $Y(\theta)$ on state $|0\rangle$, the state changes to $|q_0\rangle = cos\frac{\theta}{2}\cdot|0\rangle + sin\frac{\theta}{2}\cdot|1\rangle$. $q_0$ can also be represented as vector: $|q_0\rangle = \begin{bmatrix}\cos\frac{\theta}{2}\\ \sin\frac{\theta}{2}\end{bmatrix}$.

In this case, we have ***i)*** the amplitude of $|0\rangle$ to be $cos\frac{\theta}{2}$; ***ii)*** the amplitude of $|1\rangle$ to be $sin\frac{\theta}{2}$; ***iii)*** the probability of $P\{q_0 = |0\rangle\}$ is $cos^2\frac{\theta}{2}$; and ***iv)*** the probability of $P\{q_0 = |1\rangle\}$ is $sin^2\frac{\theta}{2}$.

### 1.2 X gate on a initialized qbit

Let $q_0$ be initialized as $|q_0\rangle = |\psi\rangle = cos\frac{\theta}{2}\cdot|0\rangle + sin\frac{\theta}{2}\cdot|1\rangle$. The X gate is to rotate $q_0$ around the X-axis by $\pi$ radians. It is equivalent to conduct operation: $X|\psi\rangle$ where $X = \begin{bmatrix}0 & 1\\ 1 & 0\end{bmatrix}$. After X gate, we have $|q_0\rangle = X|\psi\rangle = \begin{bmatrix}0 & 1\\ 1 & 0\end{bmatrix}\times\begin{bmatrix}\cos\frac{\theta}{2}\\ \sin\frac{\theta}{2}\end{bmatrix} = \begin{bmatrix}\sin\frac{\theta}{2}\\ \cos\frac{\theta}{2}\end{bmatrix}$.

In this case, ***i)*** the amplitudes of $|0\rangle$ and $|1\rangle$ are swapped; ***ii)*** the probability of $P\{q_0 = |0\rangle\}$ and $P\{q_0 = |1\rangle\}$ are swapped.

### 1.3 CNOT gate on two initialized qbits

Let $q_0$ be initialized as $|q_0\rangle = |\psi_0\rangle = \begin{bmatrix}\cos\frac{\alpha}{2}\\ \sin\frac{\alpha}{2}\end{bmatrix}$, and $q_1$ be initialized as $|q_1\rangle = |\psi_1\rangle = \begin{bmatrix}\cos\frac{\beta}{2}\\ \sin\frac{\beta}{2}\end{bmatrix}$. In CNOT operation, $q_0$ is the control qbit, whose probabilty will not be changed, but $q_1$ will be rotate around the X-axis by $\pi$ radians when $q_0$ is $|1\rangle$.

Before presenting the CNOT operation, we first introduce the combination of states $q_0$ and $q_1$ by a tensor product of $|q_0\rangle\otimes|q_1\rangle$, and we have $|q_0,q_1\rangle = |q_0\rangle\otimes|q_1\rangle = \begin{bmatrix}\cos\frac{\alpha}{2}\times\cos\frac{\beta}{2}\\ \cos\frac{\alpha}{2}\times\sin\frac{\beta}{2}\\ \sin\frac{\alpha}{2}\times\cos\frac{\beta}{2}\\ \sin\frac{\alpha}{2}\times\sin\frac{\beta}{2}\end{bmatrix}$, denoted as $\begin{bmatrix}A\\ B\\ C\\ D\end{bmatrix}$, corresponding to states $\begin{bmatrix}|00\rangle\\ |01\rangle\\ |10\rangle\\ |11\rangle\end{bmatrix}$. The matrix representation of CNOT is $\begin{bmatrix}1 & 0 & 0 & 0\\ 0 & 1 & 0 & 0\\ 0 & 0 & 0 & 1\\ 0 & 0 & 1 & 0\end{bmatrix}$. Therefore, $CNOT|q_0,q_1\rangle = \begin{bmatrix}A\\ B\\ D\\ C\end{bmatrix}$.

In this case, we can see that ***i)*** CNOT swaps the amplitude of $|10\rangle$ and $|11\rangle$. This is accordance with the definition of CNOT, where $|q_1\rangle$ is flipped when $|q_0\rangle = |1\rangle$; therefore, for original state $|11\rangle$ it changes to $|10\rangle$, likewise for original state $|10\rangle$.

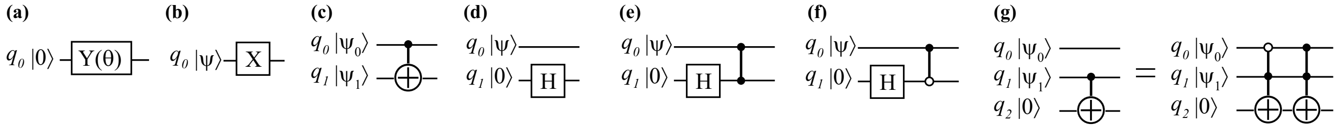


**Figure 1.** Six basic quantum gates and a pair of identity gates in QF-Circ: (a) Y gate with parameter $\theta$ to initialize qbits; (b) Pauli-X (X, or NOT) gate; (c) Controlled X (CNOT) gate to performs the NOT operation on the second qbit only when the first qbit is $|1\rangle$; (d) Hadamard (H) gate acts on qbit $q_1$ to maps the basis state $|0\rangle$ to $\frac{|0\rangle+|1\rangle}{\sqrt{2}}$; (e) Controlled Z (CZ) gate after H gate; (f) Controlled not Z (CNZ) gate after H gate; (g) identical gates.

### 1.4 H gate on $|0\rangle$ in a 2-qbits circuit

Let $q_0$ be initialized as $|\psi_0\rangle = \begin{bmatrix} \cos\frac{\alpha}{2} \\ \sin\frac{\alpha}{2} \end{bmatrix}$. Since $q_1 = |0\rangle = \begin{bmatrix} 1 \\ 0 \end{bmatrix}$, we have $|q_0, q_1\rangle = |q_0\rangle \otimes |q_1\rangle = \begin{bmatrix} \cos\frac{\alpha}{2} \\ 0 \\ \sin\frac{\alpha}{2} \\ 0 \end{bmatrix}$, denoted as $\begin{bmatrix} A \\ 0 \\ C \\ 0 \end{bmatrix}$

Applying H gate on $|q_0, q_1\rangle$ is equal to $I \otimes H|q_0, q_1\rangle$, where $I = \begin{bmatrix} 1 & 0 \\ 0 & 1 \end{bmatrix}$, $H = \frac{1}{\sqrt{2}} \begin{bmatrix} 1 & 1 \\ 1 & -1 \end{bmatrix}$, and $I \otimes H = \frac{1}{\sqrt{2}} \begin{bmatrix} 1 & 1 & 0 & 0 \\ 1 & -1 & 0 & 0 \\ 0 & 0 & 1 & 1 \\ 0 & 0 & 1 & -1 \end{bmatrix}$.

Therefore, after H gate, we have $|q_0, q_1\rangle = \frac{1}{\sqrt{2}} \begin{bmatrix} 1 & 1 & 0 & 0 \\ 1 & -1 & 0 & 0 \\ 0 & 0 & 1 & 1 \\ 0 & 0 & 1 & -1 \end{bmatrix} \times \begin{bmatrix} A \\ 0 \\ C \\ 0 \end{bmatrix} = \frac{1}{\sqrt{2}} \begin{bmatrix} A+0+0+0 \\ A+0+0+0 \\ 0+0+C+0 \\ 0+0+C+0 \end{bmatrix} = \frac{1}{\sqrt{2}} \begin{bmatrix} A \\ A \\ C \\ C \end{bmatrix}$.

In this case, we can see that the function of $H$ gate is to average the amplitude for the pair of $[|00\rangle, |01\rangle]$ and $[|10\rangle, |11\rangle]$.

### 1.5 CZ gate after H gate

We have already known the state of $|q_0, q_1\rangle$ equals $\frac{1}{\sqrt{2}} \begin{bmatrix} A \\ A \\ C \\ C \end{bmatrix}$. We also have matrix of CZ gate to be $CZ = \begin{bmatrix} 1 & 0 & 0 & 0 \\ 0 & 1 & 0 & 0 \\ 0 & 0 & 1 & 0 \\ 0 & 0 & 0 & -1 \end{bmatrix}$.

After applying CZ gate on $|q_0, q_1\rangle$, we have $CZ|q_0, q_1\rangle = \frac{1}{\sqrt{2}} \begin{bmatrix} 1 & 0 & 0 & 0 \\ 0 & 1 & 0 & 0 \\ 0 & 0 & 1 & 0 \\ 0 & 0 & 0 & -1 \end{bmatrix} \times \begin{bmatrix} A \\ A \\ C \\ C \end{bmatrix} = \frac{1}{\sqrt{2}} \begin{bmatrix} A \\ A \\ C \\ -C \end{bmatrix}$.

In this case, we can see that the function of CZ gate is to make the sign flip on the amplitude of $|11\rangle$.

### 1.6 CNZ gate after H gate

CNZ gate can be calculated as follows $CNZ = [I \otimes X]CZ[I \otimes X] = \begin{bmatrix} 1 & 0 & 0 & 0 \\ 0 & 1 & 0 & 0 \\ 0 & 0 & -1 & 0 \\ 0 & 0 & 0 & 1 \end{bmatrix}$. Similar with CZ gate, we have $CNZ|q_0, q_1\rangle = \frac{1}{\sqrt{2}} \begin{bmatrix} 1 & 0 & 0 & 0 \\ 0 & 1 & 0 & 0 \\ 0 & 0 & -1 & 0 \\ 0 & 0 & 0 & 1 \end{bmatrix} \times \begin{bmatrix} A \\ A \\ C \\ C \end{bmatrix} = \frac{1}{\sqrt{2}} \begin{bmatrix} A \\ A \\ -C \\ C \end{bmatrix}$

In this case, we can see that the function of CZ gate is to make the sign flip on the amplitude of $|10\rangle$.

### 1.7 Identical circuits

Two circuits in Figure 1(g) are identical. The first gate on the right-hand side circuit having a circle on $q_0$ and dot on $q_1$, it indicates that if $q_0 = |0\rangle$ and $q_1 = |1\rangle$, then X gate is operated on $q_0$. The second Toffoli gate indicate if $q_0 = |1\rangle$ and $q_1 = |1\rangle$, then X gate is operated on $q_0$. So, what ever $q_0 = |0\rangle$ or $q_0 = |1\rangle$, if $q_1 = |1\rangle$, then X gate is operated on $q_2$, which is the same function on the left-hand circuit.

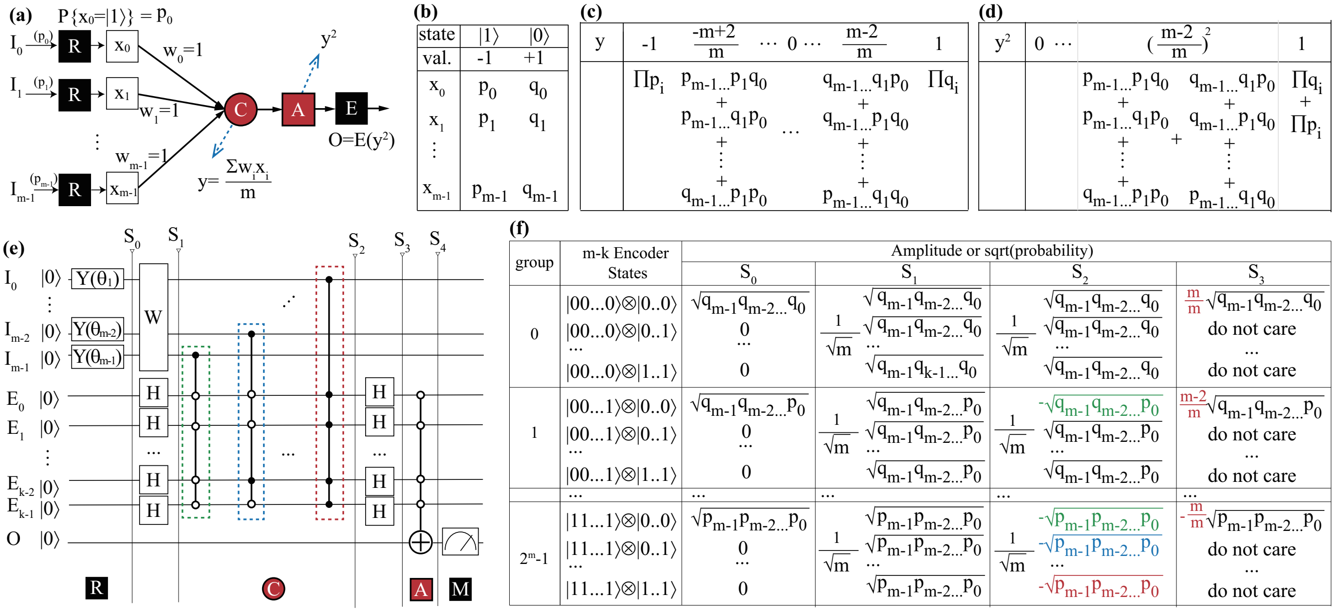


**Figure 2.** Illustration of computation at a neuron in QF-Net with the square non-linear function: (a) translation to random variables and neural computation; (b)-(d) probability distributions of random variables $x$, $y$, and $y^2$; (e) quantum circuit implementation of neural computation; (f) amplitude of states at different time steps.

## 2 Equivalency of QF-Net and QF-Circ

Based on the understandings of basic quantum gates, we now discuss the equivalency of QF-Net and QF-Circ. We will discuss neural computation and batch normalization, respectively.

### 2.1 Neural Computation

The quantum circuit design of the neural computation in Figure 2(a) is illustrated in Figure 2(e). The circuit is composed of $m$ input (I) qbits, and $k = log_2 m$ encoding (E) qbits, and 1 output (O) qbit. The $m$ input qbits and $k$ encoding qbits form a state space with $2^{m+k} = 2^m \times 2^k = m \times 2^m$ states in total. For better understanding, we divide these states into $2^m$ groups, where each group has the same $|\Phi_0\Phi_1...\Phi_{m-1}\rangle$ state for input qbits and $m$ different states for encoding qbits, as shown in 2(f). We divide the circuit into 5 steps to show the procedure: from $S_0$ to $S_4$, as shown in Figure 2(e).

At $S_0$, we initialize the circuit. For input qbit $I_k$, its initial state $\Phi_k$ is obtained by Ry gate by rotating an angle of $\theta$. According to Section 1.1, the probability of $P\{I_k = |1\rangle\} = sin^2\frac{\theta}{2}$, while $R$ operation will generate random variable $x_k$, where the probability that outcomes of $-1$ (corresponding to sate $|1\rangle$) is the given real number $p_k$. Hence, we have $sin^2\frac{\theta}{2} = p_k$, and therefore $\theta = 2 \times arcsin(\sqrt{p_k})$. For qbits in encoder from $E_0$ to $E_{k-1}$, they are initialized to $|0\rangle$. Hence, at $S_0$, only the first state in each group has amplitude; i.e., $|\Phi_0\Phi_1...\Phi_{m-1}\rangle \otimes |00...0\rangle$. The amplitude is denoted by $A_i$ for the $i^{th}$ group (e.g., $A_0 = \sqrt{q_{m-1} \cdot q_{m-2} \cdots q_0}$), as shown in Column $S_0$ in Figure 2(f). In addiion, the output qbit is initialized to $|0\rangle$.

From $S_0$ to $S_1$, we first conduct dot product of inputs and weight on input qbits. As stated in QF-Net, if $w_k = -1$, $w_k \cdot x_k$ will leas to the swap of probabilities $P\{x_k = -1\}$ and $P\{x_k = +1\}$ in $x_k$, which is equivalent to swap $P\{x_k = |1\rangle\}$ and $P\{x_k = |0\rangle\}$. X gate in Section 1.2 has exact the same function, and therefore, a $X$ gate is placed on qbit $I_k$ if and only if $W_k = -1$. For simplify of illustration, we set all weights to 1, and therefore no gates are included in $W$ component. For all encoding qbits, we apply the Hadamard ($H$) gate to make them enter superposition. From the amplitude perspective, the function of these $H$ gates will averagely distribute the amplitude in each group, as discussed in Section 1.4. The states at $S_1$ are shown in Column $S_1$ in Figure 2(f).

From $S_1$ to $S_2$, the CZ and CNZ gates are performed. As discussed in Sections 1.5 and 1.6, it will lead to the flip of sign for amplitude of specific state. As shown in Figure 2(e), each input qbit is associate to one state for the system composed of encoding qbits. Therefore, in the $i^{th}$ group where the input qbits have $n_i$ $|1\rangle$, there are $n_i$ states whose sign is flipped from "+" to "−".

From $S_2$ to $S_3$, the circuit completes the creation of all terms in the distribution of $y$. Here, we only use the information on the first state of each group, i.e., $|\Phi_0\Phi_1...\Phi_{m-1}\rangle \otimes |00...0\rangle$. The function of these $H$ gates on the first state is to accumulate all amplitude in each group and multiplies $\frac{1}{\sqrt{m}}$. As a result, for the $i^{th}$ group where $n_i$ states has flipped sign, the amplitude

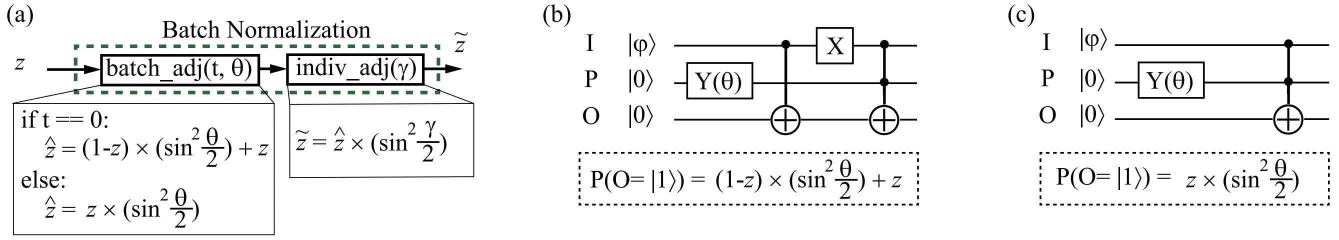


**Figure 3.** Batch normalization in QF-Net and QF-Circ: (a) functions of "batch_adj" and "indiv_adj"; (b) case $t = 0$ for batch_adj; (c) case $t = 1$ for batch_adj and indiv_ajd if $\theta$ is replaced by $\gamma$.

becomes $\frac{m-2\times n_i}{m} \times A_i$, where $A_i$ is the original amplitude for this state. We denote the amplitude as $B_i \times A_i$ Kindly note that $B_i$ is exactly the same with the corresponding value of random variable $y$ having the probability of $A_i^2$ in Figure 2(c).

Finally, from $S_3$ to $S_4$, we apply K-input controlled X gate to extract the information from encoder to output qbit $O$. According to Section 1.7, the gate adds can be expanded to $2^m$ gate by traverse all input qbits and encoding qbits, i.e., $|\Phi_0\Phi_1...\Phi_{m-1}\rangle \otimes |00...0\rangle$. For each gate, it indicates that a probability of $(B_i \times A_i)^2$ is added to qbit $O$. As a result, at $S_4$, $P\{O = |1\rangle\} = \sum_{\forall i}\{(B_i \times A_i)^2\} = (\frac{m}{m})^2 \cdot q_{m-1}q_{m-2}\cdots q_0 + (\frac{m}{m-2})^2 \cdot q_{m-1}q_{m-2}\cdots p_0 + \cdots + (-\frac{m}{m})^2 \cdot p_{m-1}p_{m-2}\cdots p_0 = E(y^2)$.

### 2.2 Batch Normalization

Figure 3 illustrates the proposed batch normalization, whose input is a real number $z$. We are going to show the equivalency of the functions in Figure 3(a) and that in Figures 3(b)-(c). First, the parameters of $t$, $\theta$, $\gamma$ are determined at training phase.

We first show that the batch_adj circuit for $t = 0$ in Figures 3(b) is equivalent to the function in Figures 3(a). In the circuit design, we have qbit $P$ for parameter and qbit $O$ for output. The qbit $P$ is initialized using a $Y$ gate with the determined parameter $\theta$, that is, its probability will be $P\{|P\rangle = |1\rangle\} = sin^2\frac{\theta}{2}$, denoted as $P_P$. The qbit $I$ is initialized as $P\{|I\rangle = |1\rangle\} = z$, $P_I$. We first apply a CNOT gate from qbit $I$ to qbit $O$; then, we apply an X gate on qbit $I$ and then a Toffoli gate using $I$ and $P$ as control. As a result, at the end of the circuit, $|O\rangle = |1\rangle$ if (1) $|I\rangle = |1\rangle$ or (2) $|I\rangle = |0\rangle$ and $|P\rangle = |1\rangle$. The probability of $P\{|O\rangle = |1\rangle\}$ is $P_I + (1-P_I) \times P_P = z + (1-z) \times = sin^2\frac{\theta}{2}$, which is the same with that in QF-Net.

We next show that the circuit in Figures 3(c) is equivalent to the function in Figures 3(a). Similar to the case of $t = 0$ in batch_adj, the qbit $P$ is initialized to have the probability of $P_P = sin^2\frac{\theta}{2}$. The qbit $I$ is initilized to have probability $P_I = z$. In this circuit, we apply a CNOT gate from qbit $I$ to qbit $O$; then, we apply a Toffoli gate on qbit $O$ using $I$ and $P$ as control. As a result, at the end of the circuit, $|O\rangle = |1\rangle$ if $|I\rangle = |1\rangle$ and $|P\rangle = |1\rangle$. The probability of $P\{|O\rangle = |1\rangle\}$ is $P_I \times P_P = z \times sin^2\frac{\theta}{2}$, which is the same with that in QF-Net.

## 3 Equivalency of Optimized 2-Input Quantum Circuits for Neural Computation

Now, we are ready to demonstrate the equivalency of four quantum circuit designs in Figure 4.

### 3.1 Design 1

In design 1 all qbits are initialized to $|0\rangle$, and then it goes through 6 step to get the final results. In the following, we will show the computing procedure of design 1.

At state $S0$: $|I_0\rangle = \begin{bmatrix}1\\0\end{bmatrix}$; $|I_1\rangle = \begin{bmatrix}1\\0\end{bmatrix}$; $|O\rangle = \begin{bmatrix}1\\0\end{bmatrix}$.

At state $S1$, $Y$ gate is applied to $|I_0\rangle$ and $|I_1\rangle$: we have $|I_0\rangle = \begin{bmatrix}cos\frac{\alpha}{2}\\sin\frac{\alpha}{2}\end{bmatrix}$; $|I_1\rangle = \begin{bmatrix}cos\frac{\beta}{2}\\sin\frac{\beta}{2}\end{bmatrix}$; $|O\rangle = \begin{bmatrix}1\\0\end{bmatrix}$, for the combination of these three qbits, we have $|I_0, I_1, O\rangle = \begin{bmatrix}\cos\frac{\alpha}{2}\times\cos\frac{\beta}{2}\\0\\\cos\frac{\alpha}{2}\times\sin\frac{\beta}{2}\\0\\\sin\frac{\alpha}{2}\times\cos\frac{\beta}{2}\\0\\\sin\frac{\alpha}{2}\times\sin\frac{\beta}{2}\\0\end{bmatrix}$, denoted as $\begin{bmatrix}A\\0\\B\\0\\C\\0\\D\\0\end{bmatrix}$.

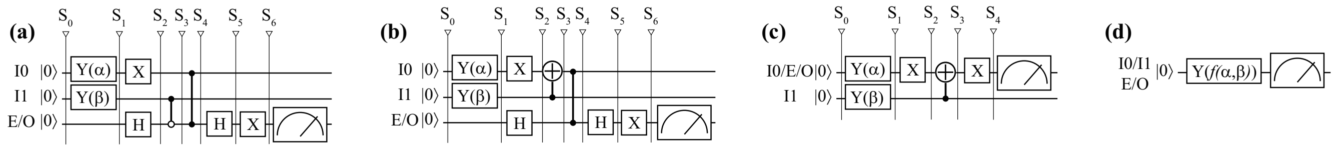


**Figure 4.** Equivalent quantum designs for 2-input neural computation: (a) design 1; (b) design 2; (c) design 3; (d) design 4.

At state $S2$, we have $|I_0, I_1, O\rangle = X \otimes I \otimes H |I_0, I_1, O\rangle = \frac{1}{\sqrt{2}} \begin{bmatrix} 0 & 0 & 0 & 0 & 1 & 1 & 0 & 0 \\ 0 & 0 & 0 & 0 & 1 & -1 & 0 & 0 \\ 0 & 0 & 0 & 0 & 0 & 0 & 1 & 1 \\ 0 & 0 & 0 & 0 & 0 & 0 & 1 & -1 \\ 1 & 1 & 0 & 0 & 0 & 0 & 0 & 0 \\ 1 & -1 & 0 & 0 & 0 & 0 & 0 & 0 \\ 0 & 0 & 1 & 1 & 0 & 0 & 0 & 0 \\ 0 & 0 & 1 & -1 & 0 & 0 & 0 & 0 \end{bmatrix} \times \begin{bmatrix} A \\ 0 \\ B \\ 0 \\ C \\ 0 \\ D \\ 0 \end{bmatrix} = \frac{1}{\sqrt{2}} \begin{bmatrix} C \\ C \\ D \\ D \\ A \\ A \\ B \\ B \end{bmatrix}$

At state $S3$, the amplitudes of $|X10\rangle$ needs a sign flip, where $X$ can be either 0 or 1; therefore, we have $|I_0, I_1, O\rangle = \frac{1}{\sqrt{2}} \begin{bmatrix} C & C & -D & D & A & A & -B & B \end{bmatrix}^T$

At state $S4$, the amplitudes of $|1X1\rangle$ needs a sign flip; therefore, we have $|I_0, I_1, O\rangle = \frac{1}{\sqrt{2}} \begin{bmatrix} C & C & -D & D & A & -A & -B & -B \end{bmatrix}^T$.

At state $S5$, we apply $I^2 \otimes H = \frac{1}{\sqrt{2}} \begin{bmatrix} 1 & 1 & 0 & 0 & 0 & 0 & 0 & 0 \\ 1 & -1 & 0 & 0 & 0 & 0 & 0 & 0 \\ 0 & 0 & 1 & 1 & 0 & 0 & 0 & 0 \\ 0 & 0 & 1 & -1 & 0 & 0 & 0 & 0 \\ 0 & 0 & 0 & 0 & 1 & 1 & 0 & 0 \\ 0 & 0 & 0 & 0 & 1 & -1 & 0 & 0 \\ 0 & 0 & 0 & 0 & 0 & 0 & 1 & 1 \\ 0 & 0 & 0 & 0 & 0 & 0 & 1 & -1 \end{bmatrix}$ on $|I_0, I_1, O\rangle$. We have $|I_0, I_1, O\rangle = \begin{bmatrix} C \\ 0 \\ 0 \\ -D \\ 0 \\ A \\ -B \\ 0 \end{bmatrix}$

At state $S6$, we apply $I^2 \otimes X = \begin{bmatrix} 0 & 1 & 0 & 0 & 0 & 0 & 0 & 0 \\ 1 & 0 & 0 & 0 & 0 & 0 & 0 & 0 \\ 0 & 0 & 0 & 1 & 0 & 0 & 0 & 0 \\ 0 & 0 & 1 & 0 & 0 & 0 & 0 & 0 \\ 0 & 0 & 0 & 0 & 0 & 1 & 0 & 0 \\ 0 & 0 & 0 & 0 & 1 & 0 & 0 & 0 \\ 0 & 0 & 0 & 0 & 0 & 0 & 0 & 1 \\ 0 & 0 & 0 & 0 & 0 & 0 & 1 & 0 \end{bmatrix}$, and we have $|I_0, I_1, O\rangle = \begin{bmatrix} 0 \\ C \\ -D \\ 0 \\ A \\ 0 \\ 0 \\ -B \end{bmatrix}$

Finally, we only measure qbit $O$, which indicate all probability of $|XX1\rangle$ will be sum up. So, the final output probability is $C^2 + (-B)^2 = C^2 + B^2$.

## 3.2 Design 2

In design 2, only operation between $S_2$ and $S_3$ is changed.

We can take use of the previous results at $S_2$, where $|I_0, I_1, O\rangle = \frac{1}{\sqrt{2}} \begin{bmatrix} C & C & D & D & A & A & B & B \end{bmatrix}^T$.

At $S3$, we apply $CNOT$ on $I_0$ controller by $I_1$, indicating all $|X1Y\rangle$ will be swapped to $|\hat{X}1Y\rangle$, where $X = 0$ then $\hat{X} = 1$ or $X = 1$ then $\hat{X} = 0$. Hence, $|I_0, I_1, O\rangle = \frac{1}{\sqrt{2}} \begin{bmatrix} C & C & B & B & A & A & D & D \end{bmatrix}^T$, where B and D swapped.

At $S4$, the amplitudes of $|1X1\rangle$ needs a sign flip; therefore, we have $|I_0, I_1, O\rangle = \frac{1}{\sqrt{2}} \begin{bmatrix} C & C & B & B & A & -A & D & -D \end{bmatrix}^T$.

At $S5$, we will have $|I_0, I_1, O\rangle = \begin{bmatrix} C & 0 & B & 0 & 0 & A & 0 & D \end{bmatrix}^T$ Then, at $S6$, we have $|I_0, I_1, O\rangle = \begin{bmatrix} 0 & C & 0 & B & A & 0 & D & 0 \end{bmatrix}^T$

When we measure qbit $O$, we can also obtain $C^2 + B^2$.

## 3.3 Design 3

For design 3, we merge qbit $O$ to $I0$.

At $S1$, we have $|I_0, I_1, O\rangle = \begin{bmatrix} \cos\frac{\alpha}{2} \times \cos\frac{\beta}{2} & \cos\frac{\alpha}{2} \times \sin\frac{\beta}{2} & \sin\frac{\alpha}{2} \times \cos\frac{\beta}{2} & \sin\frac{\alpha}{2} \times \sin\frac{\beta}{2} \end{bmatrix}^T = \begin{bmatrix} A & B & C & D \end{bmatrix}^T$.

Then at $S2$, X gate is applied to $I0$, we swap $A, B$ and $C, D$ to obtain $|I_0, I_1, O\rangle = \begin{bmatrix} C & D & B & A \end{bmatrix}^T$.

Next, at $S3$, CNOT gate is applied to $I0$ controlled by $I1$, hence we swap $D$ and $B$ to obtain $|I_0, I_1, O\rangle = \begin{bmatrix} C & B & A & D \end{bmatrix}^T$.

At $S4$, X gate is applied to $I0$, we swap $C,B$ and $A,D$ to obtain $|I_0,I_1,O\rangle = \begin{bmatrix} A & D & C & B \end{bmatrix}^T$.

Finally, we measure $I0$ which involve the amplitude marked red at $S4$, and we obtain the output probability of $C^2+B^2$.

### 3.4 Design 4

For design 4, we take another angle to derive it from design 3.

For design 3, at $S1$ the probability of $P\{I_0 = |1\rangle\}$ is $x = sin^2\frac{\alpha}{2}$, while that of $P\{I_1 = |1\rangle\}$ is $y = sin^2\frac{\beta}{2}$.

At $S2$, the $X$ gate is applied, so the probability of $P\{I_0 = |1\rangle\}$ changes to $1-x = cos^2\frac{\alpha}{2}$, and $P\{I_0 = |0\rangle\} = x$.

Then at $S3$, if $I_1 = |1\rangle$, $I_0$ will flip. We know that the probability of $P\{I_1 = |1\rangle\} = y$, so $P\{I_0 = |0\rangle, I_1 = |1\rangle\} = y \times x$ and $P\{I_0 = |1\rangle, I_1 = |1\rangle\} = y \times (1-x)$. After this step, the probability of $P\{I_0 = |1\rangle\}$ changes to $1-x+y\times x-y\times(1-x) = 1-x-y+2\cdot x\cdot y$.

Finally, at $S4$, we flip $I_0$ again, and the probability of $P\{I_0 = |1\rangle\}$ changes to $1-[1-x-y+2xy] = x+y-2\cdot x\cdot y$.

Since $x$ and $y$ are inputs which are known at beginning, we can directly initialize qbit $I_0$ to obtain the above probability by creating a function $f(\alpha,\beta)$. Let $z = f(\alpha,\beta)$, we know the output probability of design 4 is $sin^2\frac{z}{2}$. We then let $sin^2\frac{z}{2} = x+y-2\cdot x\cdot y$, and we can derive $z = 2\cdot arcsin(\sqrt{x+y-2\cdot x\cdot y})$.
